# Supplementary material for: Plane Geometry Problem Solving with Multi-modal Reasoning: A Survey
Source: arXiv:2505.14340 source file (2025-05-20)
Supplement: Supplementary file 1 [file PGPS_datasets.tex]

\section{PGPS Datasets}

\subsection{Summary of PGPS datasets}

\begin{table*}[t]
    \centering
    \resizebox{\linewidth}{!}{
    \begin{tabular}{llp{0.4\linewidth}}
        \toprule
        \textbf{Input–output format} & \textbf{Collection method} & \textbf{Datasets and benchmarks} \\
        \midrule
        Problem to scalar value or choice & Human annotation & GEOS~\citep{geos}, GeoShader~\citep{GeoShader}, Geometry3K~\citep{intergps}, GeoQA~\citep{geoqa}, GeoQA+~\citep{geoqa+}, PGPS9K~\citep{pgps9k}, formalgeo7k~\citep{formalgeo7k}, MathVerse~\citep{mathverse}, MathVista~\citep{mathvista}, MMMU~\citep{mmmu}, MATH-V~\citep{Math-Vision}, DynaMath~\citep{dynamath}, GeoSense~\citep{geosense}, VCBench~\citep{vcbench}, PolyMath~\citep{polymath} \\
        & Synthetic annotation & GeoTrust~\citep{TrustGeoGen}, GeomVerse~\citep{geomverse}, VisOnlyQA~\citep{visonlyqa} \\
        % \multirow{2}{*}{Benchmark only} 
        %     & Human annotation & GeoShader, MathVerse, MathVista, MMMU, MATH-V, DynaMath, GeoSense, VCBench, PolyMath \\
        %     & Synthetic annotation & GeoTrust,\;GeomVerse,\;VisOnlyQA \\
        \midrule
        Diagram to formal-language description 
            & Human annotation & GEOS~\citep{geos}, GEOS++~\citep{geos++}, GEOS-OS~\citep{GEOS-OS}, Geometry3K~\citep{intergps}, PGDP5K~\citep{pgdp5k}, PGPS9K~\citep{pgps9k}, formalgeo7k~\citep{formalgeo7k} \\
        \midrule
        Formal-language description to theorem sequences 
            & Human annotation & GEOS++~\citep{geos++}, GEOS-OS~\citep{GEOS-OS}, Geometry3K~\citep{intergps}, formalgeo7k~\citep{formalgeo7k} \\
        \midrule
        Problem to logic program 
            & Human annotation & GeoQA~\citep{geoqa}, GeoQA+~\citep{geoqa+}, PGPS9K~\citep{pgps9k}, UniGeo~\citep{unigeo} \\
        \midrule
        Problem to natural-language description & L(V)LM-assisted annotation & G-LLaVA~\citep{G-LLaVA}, MATH-LLaVA~\citep{math-llava}, GPSM4K~\citep{GPSM4K}, MAVIS~\citep{mavis} \\
        & Synthetic annotation & MAVIS~\citep{mavis}, GeoDANO~\citep{GeoDANO} \\
        % \multirow{2}{*}{Problem $\rightarrow$ natural-language description} 
        %     & L(V)LM-assisted annotation & G-LLaVA, MATH-LLaVA, GPSM4K, MAVIS \\
        %     & Synthetic annotation & MAVIS \\
        \bottomrule
    \end{tabular}
    }
    \caption{Summary of input-output formats, collection methods, and associated PGPS datasets and benchmarks. We categorize the existing PGPS datasets and benchmarks based on the input-output format and the collection strategy.}
    \label{tab:dataset_overview}
\end{table*}

% \begin{table*}[t!]
% \centering
% \resizebox{\linewidth}{!}{
% \begin{tabular}{lp{8cm}}
% \toprule
% \textbf{Datasets} & \textbf{Sources of diagrams} \\
% \midrule
% G\textendash{}LLaVA~\citep{G-LLaVA} & GeoQA$+$, Geometry3K \\
% MAVIS~\citep{mavis} & Synthetic; Geometry3K, GeoQA$+$; 4{,}000 manually collected problems \\
% Math\textendash{}LLaVA~\citep{math-llava} & GEOS, GeoQA$+$, Geometry3K, UniGeo \\
% CogAlign~\citep{CogAlign} & Synthetic \\
% VisOnlyQA~\citep{visonlyqa} & Synthetic \\
% GPSM4K~\citep{GPSM4K} & \\
% \midrule
% \textbf{Benchmarks} & \textbf{Sources of problems} \\
% \midrule
% MMMU~\citep{mmmu}          & Unknown \\
% Math\textendash V~\citep{Math-Vision}      & 19 competitions (e.g., AMC 8, 10, 12) \\
% MathVista~\citep{mathvista}      & GEOS, GeoQA$+$, Geometry3K, UniGeo \\
% MathVerse~\citep{mathverse}      & GeoQA, GEOS, Geometry3K; plus 370 manually collected from internet \\
% GeomVerse~\citep{geomverse}      & Synthetic (algorithmically generated) \\
% DynaMath~\citep{dynamath}       & Seeded from Math\textendash V \\
% VisOnlyQA~\citep{visonlyqa}      & Synthetic \\
% MM\textendash MATH~\citep{mm-math}      & 21st Century Education Network \\
% GeoEval~\citep{geoeval}        & Geometry3K, PGPS9K, UniGeo, GeoQA$+$ \\
% \bottomrule
% \end{tabular}
% }
% \end{table*}

We summarize the PGPS datasets and benchmarks in the perspective of input-output format and the collection method at \cref{tab:dataset_overview}.
